# Supplementary material for: Meent: Differentiable Electromagnetic Simulator for Machine Learning
Source: arXiv:2406.12904 source file (2024-06-11)
Supplement: Supplementary file 1 [file datasheet.tex]

\subsection{Motivation}

The questions in this section are primarily intended to encourage
dataset creators to clearly articulate their reasons for creating the
dataset and to promote transparency about funding interests.
The latter may be particularly relevant for datasets created for
research purposes.\\

\begin{itemize}

\item \textbf{For what purpose was the dataset created?} Was there a specific task in mind? Was there a specific gap that needed to be filled? Please provide a description.

\item \textbf{Who created the dataset (e.g., which team, research group) and on behalf of which entity (e.g., company, institution, organization)?}

\item \textbf{Who funded the creation of the dataset?} If there is an associated grant, please provide the name of the grantor and the grant name and number.

\item \textbf{Any other comments?}

\end{itemize}

\subsection{Composition}

Dataset creators should read through \edit{these questions} prior to
any data collection and then provide answers once \edit{data} collection is
complete. Most of the questions \edit{in this section} are intended to
provide dataset consumers with the information they need to make
informed decisions about using the dataset for their chosen
tasks. Some of the questions are \edit{designed to elicit} information
about compliance with the EU's General Data Protection Regulation
(GDPR) or comparable regulations in other jurisdictions.

\edit{Questions that apply only to datasets that relate to people are
grouped together at the end of the section. We recommend taking a
broad interpretation of whether a dataset relates to people. For
example, any dataset containing text that was written by people
relates to people.}\\

\begin{itemize}

\item \textbf{What do the instances that comprise the dataset
    represent (e.g., documents, photos, people, countries)?} Are there
  multiple types of instances (e.g., movies, users, and ratings;
  people and interactions between them; nodes and edges)? Please
  provide a description.

\item \textbf{How many instances are there in total (of each type, if appropriate)?}

\item \textbf{Does the dataset contain all possible instances or is it
    a sample (not necessarily random) of instances from a larger set?}
  If the dataset is a sample, then what is the larger set? Is the
  sample representative of the larger set (e.g., geographic coverage)?
  If so, please describe how this representativeness was
  validated/verified. If it is not representative of the larger set,
  please describe why not (e.g., to cover a more diverse range of
  instances, because instances were withheld or unavailable).

\item \textbf{What data does each instance consist of?} ``Raw'' data
  (e.g., unprocessed text or images) or features? In either case,
  please provide a description.

\item \textbf{Is there a label or target associated with each
    instance?} If so, please provide a description.

\item \textbf{Is any information missing from individual instances?}
  If so, please provide a description, explaining why this information
  is missing (e.g., because it was unavailable). This does not include
  intentionally removed information, but might include, e.g., redacted
  text.

\item \textbf{Are relationships between individual instances made
    explicit (e.g., users' movie ratings, social network links)?} If
  so, please describe how these relationships are made explicit.

\item \textbf{Are there recommended data splits (e.g., training,
    development/validation, testing)?} If so, please provide a
  description of these splits, explaining the rationale behind them.

\item \textbf{Are there any errors, sources of noise, or redundancies
    in the dataset?} If so, please provide a description.

\item \textbf{Is the dataset self-contained, or does it link to or
    otherwise rely on external resources (e.g., websites, tweets,
    other datasets)?} If it links to or relies on external resources,
    a) are there guarantees that they will exist, and remain constant,
    over time; b) are there official archival versions of the complete
    dataset (i.e., including the external resources as they existed at
    the time the dataset was created); c) are there any restrictions
    (e.g., licenses, fees) associated with any of the external
    resources that might apply to a \edit{dataset consumer}? Please provide
    descriptions of all external resources and any restrictions
    associated with them, as well as links or other access points, as
    appropriate.

\item \textbf{Does the dataset contain data that might be considered
    confidential (e.g., data that is protected by legal privilege or
    by doctor\edit{--}patient confidentiality, data that includes the content
    of individuals' non-public communications)?} If so, please provide
    a description.

\item \textbf{Does the dataset contain data that, if viewed directly,
    might be offensive, insulting, threatening, or might otherwise
    cause anxiety?} If so, please describe why.

\end{itemize}

% \edit{If the dataset does not }relate to people, you may skip the remaining questions in this section.

% \begin{itemize}

% \item \textbf{Does the dataset identify any subpopulations (e.g., by
%     age, gender)?} If so, please describe how these subpopulations are
%   identified and provide a description of their respective
%   distributions within the dataset.

% \item \textbf{Is it possible to identify individuals (i.e., one or
%     more natural persons), either directly or indirectly (i.e., in
%     combination with other data) from the dataset?} If so, please
%     describe how.

% \item \textbf{Does the dataset contain data that might be considered
%     sensitive in any way (e.g., data that reveals rac\edit{e} or ethnic
%     origins, sexual orientations, religious beliefs, political
%     opinions or union memberships, or locations; financial or health
%     data; biometric or genetic data; forms of government
%     identification, such as social security numbers; criminal
%     history)?} If so, please provide a description.

% \item \textbf{Any other comments?}

% \end{itemize}

\subsection{Collection Process}

As with the \edit{questions in the} previous section, dataset creators should
read through these questions prior to any data collection to flag
potential issues and then provide answers once collection is complete.
\edit{In addition to the goals outlined in the previous section, the
questions in this section are designed to elicit information that may
help researchers and practitioners to create alternative datasets with
similar characteristics. Again, questions that apply only to datasets
that relate to people are grouped together at the end of the
section.}\\

\begin{itemize}

\item \textbf{How was the data associated with each instance
    acquired?} Was the data directly observable (e.g., raw text, movie
  ratings), reported by subjects (e.g., survey responses), or
  indirectly inferred/derived from other data (e.g., part-of-speech
  tags, model-based guesses for age or language)? If \edit{the} data was reported
  by subjects or indirectly inferred/derived from other data, was the
  data validated/verified? If so, please describe how.

\item \textbf{What mechanisms or procedures were used to collect the
    data (e.g., hardware apparatus\edit{es} or sensor\edit{s}, manual human
    curation, software program\edit{s}, software API\edit{s})?} How were these
    mechanisms or procedures validated?

\item \textbf{If the dataset is a sample from a larger set, what was
    the sampling strategy (e.g., deterministic, probabilistic with
    specific sampling probabilities)?}

\item \textbf{Who was involved in the data collection process (e.g.,
    students, crowdworkers, contractors) and how were they compensated
    (e.g., how much were crowdworkers paid)?}

\item \textbf{Over what timeframe was the data collected?} Does this
  timeframe match the creation timeframe of the data associated with
  the instances (e.g., recent crawl of old news articles)?  If not,
  please describe the timeframe in which the data associated with the
  instances was created.

\item \textbf{Were any ethical review processes conducted (e.g., by an
    institutional review board)?} If so, please provide a description
  of these review processes, including the outcomes, as well as a link
  or other access point to any supporting documentation.

\end{itemize}

\edit{If the dataset does not relate to people, you may skip the remaining questions in this section.}

\begin{itemize}

\item \textbf{Did you collect the data from the individuals in
    question directly, or obtain it via third parties or other sources
    (e.g., websites)?}

\item \textbf{Were the individuals in question notified about the data
    collection?} If so, please describe (or show with screenshots or
  other information) how notice was provided, and provide a link or
  other access point to, or otherwise reproduce, the exact language of
  the notification itself.

\item \textbf{Did the individuals in question consent to the
    collection and use of their data?} If so, please describe (or show
  with screenshots or other information) how consent was requested and
  provided, and provide a link or other access point to, or otherwise
  reproduce, the exact language to which the individuals consented.

\item \textbf{If consent was obtained, were the consenting individuals
    provided with a mechanism to revoke their consent in the future or
    for certain uses?} If so, please provide a description, as well as
  a link or other access point to the mechanism (if appropriate).

\item \textbf{Has an analysis of the potential impact of the dataset
    and its use on data subjects (e.g., a data protection impact
    analysis) been conducted?} If so, please provide a description of
  this analysis, including the outcomes, as well as a link or other
  access point to any supporting documentation.

\item \textbf{Any other comments?}

\end{itemize}

\subsection{Preprocessing/cleaning/labeling}

Dataset creators should read through these questions prior to any
preprocessing, cleaning, or labeling and then provide answers once
these tasks are complete. The questions in this section are intended
to provide dataset consumers with the information they need to
determine whether the ``raw'' data has been processed in ways that are
compatible with their chosen tasks. For example, text that has been
converted into a ``bag-of-words'' is not suitable for tasks involving
word order.\\

\begin{itemize}

\item \textbf{Was any preprocessing/cleaning/labeling of the data done
    (e.g., discretization or bucketing, tokenization, part-of-speech
    tagging, SIFT feature extraction, removal of instances, processing
    of missing values)?} If so, please provide a description. If not,
  you may skip the remain\edit{ing} questions in this section.

\item \textbf{Was the ``raw'' data saved in addition to the preprocessed/cleaned/labeled data (e.g., to support unanticipated future uses)?} If so, please provide a link or other access point to the ``raw'' data.

\item \textbf{Is the software \edit{that was} used to preprocess/clean/label the \edit{data} available?} If so, please provide a link or other access point.

\item \textbf{Any other comments?}

\end{itemize}

\subsection{Uses}

\edit{The} questions \edit{in this section} are intended to encourage dataset
creators to reflect on the tasks for which the dataset should and
should not be used. By explicitly highlighting these tasks, dataset
creators can help dataset consumers to make informed decisions,
thereby avoiding potential risks or harms.\\

\begin{itemize}

\item \textbf{Has the dataset been used for any tasks already?} If so, please provide a description.

\item \textbf{Is there a repository that links to any or all papers or systems that use the dataset?} If so, please provide a link or other access point.

\item \textbf{What (other) tasks could the dataset be used for?}

\item \textbf{Is there anything about the composition of the dataset or the way it was collected and preprocessed/cleaned/labeled that might impact future uses?} For example, is there anything that a \edit{dataset consumer} might need to know to avoid uses that could result in unfair treatment of individuals or groups (e.g., stereotyping, quality of service issues) or other \edit{risks or} harms (e.g., \edit{legal risks,} financial harms\edit{)?} If so, please provide a description. Is there anything a \edit{dataset consumer} could do to mitigate these \edit{risks or} harms?

\item \textbf{Are there tasks for which the dataset should not be used?} If so, please provide a description.

\item \textbf{Any other comments?}

\end{itemize}

\subsection{Distribution}

Dataset creators should provide answers to these questions prior to
distributing the dataset either internally within the entity on behalf
of which the dataset was created or externally to third parties.\\

\begin{itemize}

\item \textbf{Will the dataset be distributed to third parties outside of the entity (e.g., company, institution, organization) on behalf of which the dataset was created?} If so, please provide a description.

\item \textbf{How will the dataset will be distributed (e.g., tarball on website, API, GitHub)?} Does the dataset have a digital object identifier (DOI)?

\item \textbf{When will the dataset be distributed?}

\item \textbf{Will the dataset be distributed under a copyright or other intellectual property (IP) license, and/or under applicable terms of use (ToU)?} If so, please describe this license and/or ToU, and provide a link or other access point to, or otherwise reproduce, any relevant licensing terms or ToU, as well as any fees associated with these restrictions.

\item \textbf{Have any third parties imposed IP-based or other restrictions on the data associated with the instances?} If so, please describe these restrictions, and provide a link or other access point to, or otherwise reproduce, any relevant licensing terms, as well as any fees associated with these restrictions.

\item \textbf{Do any export controls or other regulatory restrictions apply to the dataset or to individual instances?} If so, please describe these restrictions, and provide a link or other access point to, or otherwise reproduce, any supporting documentation.

\item \textbf{Any other comments?}

\end{itemize}

\subsection{Maintenance}

As with the \edit{questions in the} previous section, dataset creators
should provide answers to these questions prior to distributing the
dataset. The questions \edit{in this section} are intended to
encourage dataset creators to plan for dataset maintenance and
communicate this plan \edit{to} dataset consumers.\\

\begin{itemize}

\item \textbf{Who \edit{will be} supporting/hosting/maintaining the dataset?}

\item \textbf{How can the owner/curator/manager of the dataset be contacted (e.g., email address)?}

\item \textbf{Is there an erratum?} If so, please provide a link or other access point.

\item \textbf{Will the dataset be updated (e.g., to correct labeling
    errors, add new instances, delete instances)?} If so, please
  describe how often, by whom, and how updates will be communicated to
  \edit{dataset consumers} (e.g., mailing list, GitHub)?

\item \textbf{If the dataset relates to people, are there applicable
    limits on the retention of the data associated with the instances
    (e.g., were \edit{the} individuals in question told that their data would
    \edit{be} retained for a fixed period of time and then deleted)?} If so,
    please describe these limits and explain how they will be
    enforced.

\item \textbf{Will older versions of the dataset continue to be
    supported/hosted/maintained?} If so, please describe how. If not,
  please describe how its obsolescence will be communicated to \edit{dataset
  consumers}.

\item \textbf{If others want to extend/augment/build on/contribute to
    the dataset, is there a mechanism for them to do so?} If so,
  please provide a description. Will these contributions be
  validated/verified? If so, please describe how. If not, why not? Is
  there a process for communicating/distributing these contributions
  to \edit{dataset consumers}? If so, please provide a description.

\item \textbf{Any other comments?}

\end{itemize}
